# Supplementary material for: Explicit Quantum Circuits for Block Encodings of Certain Sparse Matrices
Source: arXiv:2203.10236 source file (2023-05-22)
Supplement: Supplementary file 1 [file supplement.tex]

% SIAM Supplemental File Template
\documentclass[review,supplement,hidelinks,onefignum,onetabnum]{siamart220329}

\input{shared}

\externaldocument[][nocite]{main}

% Optional PDF information
\ifpdf
\hypersetup{
  pdftitle={Supplementary Materials: Quantum Circuits for Block Encodings},
  pdfauthor={D. Camps, L. Lin, R. Van Beeumen, and C. Yang}
}
\fi

\begin{document}

\maketitle

\input appendix.tex

\bibliographystyle{siamplain}
\bibliography{references}

\end{document}
